# Supplementary material for: Sentiment Analysis through LLM Negotiations
Source: arXiv:2311.01876 source file (2023-11-03)
Supplement: Supplementary file 1 [file appendix_case.tex]

\begin{table*}
\label{tab:methods}
\centering
\small
\vskip 0.1in
\scalebox{0.95}{
\begin{tabular}{ll}
    \toprule
    \multicolumn{2}{c}{\bf SST-2 : positive/negative sentiment analysis} \\
    \toprule
    {\bf \textit{Label Word Map}} & \{0: Negative, 1: Positive\} \\\midrule
    {\bf \textit{Zero-Shot}} & \\
    \specialrule{0em}{1pt}{1pt}
    \cdashline{1-2}
    \specialrule{0em}{1pt}{1pt}
    Classify Prompt: & Please classify the overall SENTIMENT polarity of the INPUT sentence as Positive or Negative. \\ 
    & INPUT: <sent> \\
    & SENTIMENT:  \\
    %& \text{} \\
    \specialrule{0em}{1pt}{1pt}
    \cdashline{1-2}
    \specialrule{0em}{1pt}{1pt}
    Reason-Classify Prompts: & Please classify the overall SENTIMENT polarity of the INPUT sentence as Positive or Negative. \\
    & INPUT: <sent> \\
    & \text{} \\
    \specialrule{0em}{1pt}{1pt}
    \cdashline{1-2}
    \specialrule{0em}{1pt}{1pt}
    Findclue-Reason-Classify & {\bf Step 1:} \\
    & Please classify the overall SENTIMENT polarity of the INPUT sentence as Positive or Negative.\\ 
    & INPUT: <sent> \\
    & \text{} \\
    & {\bf Step 2:}\\ 
    & Please classify the overall SENTIMENT polarity of the INPUT sentence as Positive or Negative. \\ 
    & INPUT: <sent> \\
    & CLUES: <step-1-response>\\
    & \text{} \\
    \midrule
    %%%%%%%%%%%%%%%%%%%%%%%%%%%%%%%%
    % few-shot 
    %%%%%%%%%%%%%%%%%%%%%%%%%%%%%%%%%
    {\bf \textit{Few-Shot}} & \\
    \specialrule{0em}{1pt}{1pt}
    \cdashline{1-2}
    \specialrule{0em}{1pt}{1pt}
    Classify Prompt: & Please classify the overall SENTIMENT polarity of the INPUT sentence as Positive or Negative. \\ 
    & INPUT: <demo-sent> \\
    & SENTIMENT: <demo-label-word> \\
    & \text{} \\
    & INPUT: <demo-sent> \\
    & SENTIMENT: <demo-label-word> \\
    & \text{} \\
    & INPUT: <sent> \\
    & SENTIMENT:  \\
    \specialrule{0em}{1pt}{1pt}
    \cdashline{1-2}
    \specialrule{0em}{1pt}{1pt}
    Reason-Classify Prompts: &  {\bf Step 1:}\\
    & Classify the sentiment of the input sentence as positive or negative. \\
    & INPUT: <demo-sent> \\
    & \text{} \\
    & {\bf Step 2:} \\ 
    & Classify the sentiment of the input sentence as positive or negative.  \\
    & \text{} \\
    & INPUT: <demo-sent> \\
    & REASONING: <step-1-generated>\\ 
    & SENTIMENT: <demo-label-word>\\
    & \text{} \\
    & INPUT: <demo-sent> \\
    & REASONING: <step-1-generated>\\ 
    & SENTIMENT: <demo-label-word>\\
    & \text{} \\
    & INPUT: <test-sent> \\
    \specialrule{0em}{1pt}{1pt}
    \cdashline{1-2}
    \specialrule{0em}{1pt}{1pt}
    Findclue-Reason-Classify Prompts: &  {\bf Step 1:}\\
    & Classify the sentiment of the input sentence as positive or negative. \\
    & INPUT: <demo-sent> \\
    & \text{} \\
    & {\bf Step 2:} \\ 
    & Classify the sentiment of the input sentence as positive or negative.  \\
    & \text{} \\
    & INPUT: <demo-sent> \\
    & REASONING: <step-1-generated>\\ 
    & SENTIMENT: <demo-label-word>\\
    & \text{} \\
    & INPUT: <demo-sent> \\
    & REASONING: <step-1-generated>\\ 
    & SENTIMENT: <demo-label-word>\\
    & \text{} \\
    & INPUT: <test-sent> \\
    %%%%%%%%%%%%%%%%%%%%%
    %\midrule
    \bottomrule
\end{tabular}
}
\caption{Examples of prompts for setups in Section~\ref{sec:methods}.}
\label{example:prompt_sst2}
\end{table*}
